# Supplementary material for: Plasmons in phosphorene nanoribbons
Source: arXiv:2305.09532 source file (2023-05-16)
Supplement: Supplementary file 1 [file supplement.tex]

\documentclass[%
%reprint,
superscriptaddress,
%groupedaddress,
%unsortedaddress,
%runinaddress,
%frontmatterverbose, 
%preprint,
%showpacs,preprintnumbers,
nofootinbib,
%nobibnotes,
%bibnotes,
amsmath,amssymb,
aps,
pra,
onecolumn,%twocolumn,
%prb,
%rmp,
%prstab,
%prstper,
%floatfix,
%secnumarabic
]{revtex4-2}

\usepackage{amsmath}
\usepackage{amssymb}
\usepackage{amsfonts}
\usepackage{bm} % bold math
\usepackage{bbm}
\usepackage{braket}
\usepackage{color}
\usepackage{comment}
\usepackage{dcolumn} % align table columns on decimal point
\usepackage{dsfont}
\usepackage{enumerate}
\usepackage{epsfig}
\usepackage{esint}
\usepackage[T1]{fontenc}
\usepackage{framed}
\usepackage{textcomp, gensymb}
\usepackage{graphicx} % include figure files
\usepackage[colorlinks,linkcolor=blue,citecolor=blue,urlcolor=blue,hyperindex,driverfallback=dvipdfm]{hyperref}
\usepackage{indentfirst}
\usepackage{lmodern}
\usepackage{mathrsfs}
\usepackage{mathtools}
\usepackage{multirow}
\usepackage{psfrag}
\usepackage{pst-all}
\usepackage{soul}
\usepackage{units}
\usepackage{xcolor}
\usepackage{xspace}

\mathtoolsset{showonlyrefs} % label only referred equations

\begin{document}

\title{Plasmons in phosphorene nanoribbons \\ {\color{gray} \small -- SUPPLEMENTAL MATERIAL --}}

\author{Line Jelver}
\email[Line Jelver: ]{lije@mci.sdu.dk}
\affiliation{POLIMA---Center for Polariton-driven Light--Matter Interactions, University of Southern Denmark, Campusvej 55, DK-5230 Odense M, Denmark}

\author{Joel~D.~Cox}
\email[Joel~D.~Cox: ]{cox@mci.sdu.dk}
\affiliation{POLIMA---Center for Polariton-driven Light--Matter Interactions, University of Southern Denmark, Campusvej 55, DK-5230 Odense M, Denmark}
\affiliation{Danish Institute for Advanced Study, University of Southern Denmark, Campusvej 55, DK-5230 Odense M, Denmark}

\begin{abstract}
We present first-principles calculations of the electronic band structure for the phosphorene nanoribbons considered in the main text, where the results obtained using different density functional theory (DFT) codes are compared. We additionally show second-principles optical response calculations in the noninteracting limit (i.e., neglecting electron-electron interactions), comparing results based on the Wannier tight-binding Hamiltonian to equivalent calculations obtained directly from DFT wavefunctions.
\end{abstract}

\date{\today}
\maketitle
%\tableofcontents

%%%%%%%%%%%%%%%%%%%%%%%%%%%%%%%%%%%%%%%%%%%%%%%%%%%%%%%%%%%%%%%%%%%%%%%%%%%%%%%

\begin{figure}
    \centering
    \includegraphics[width=1\textwidth]{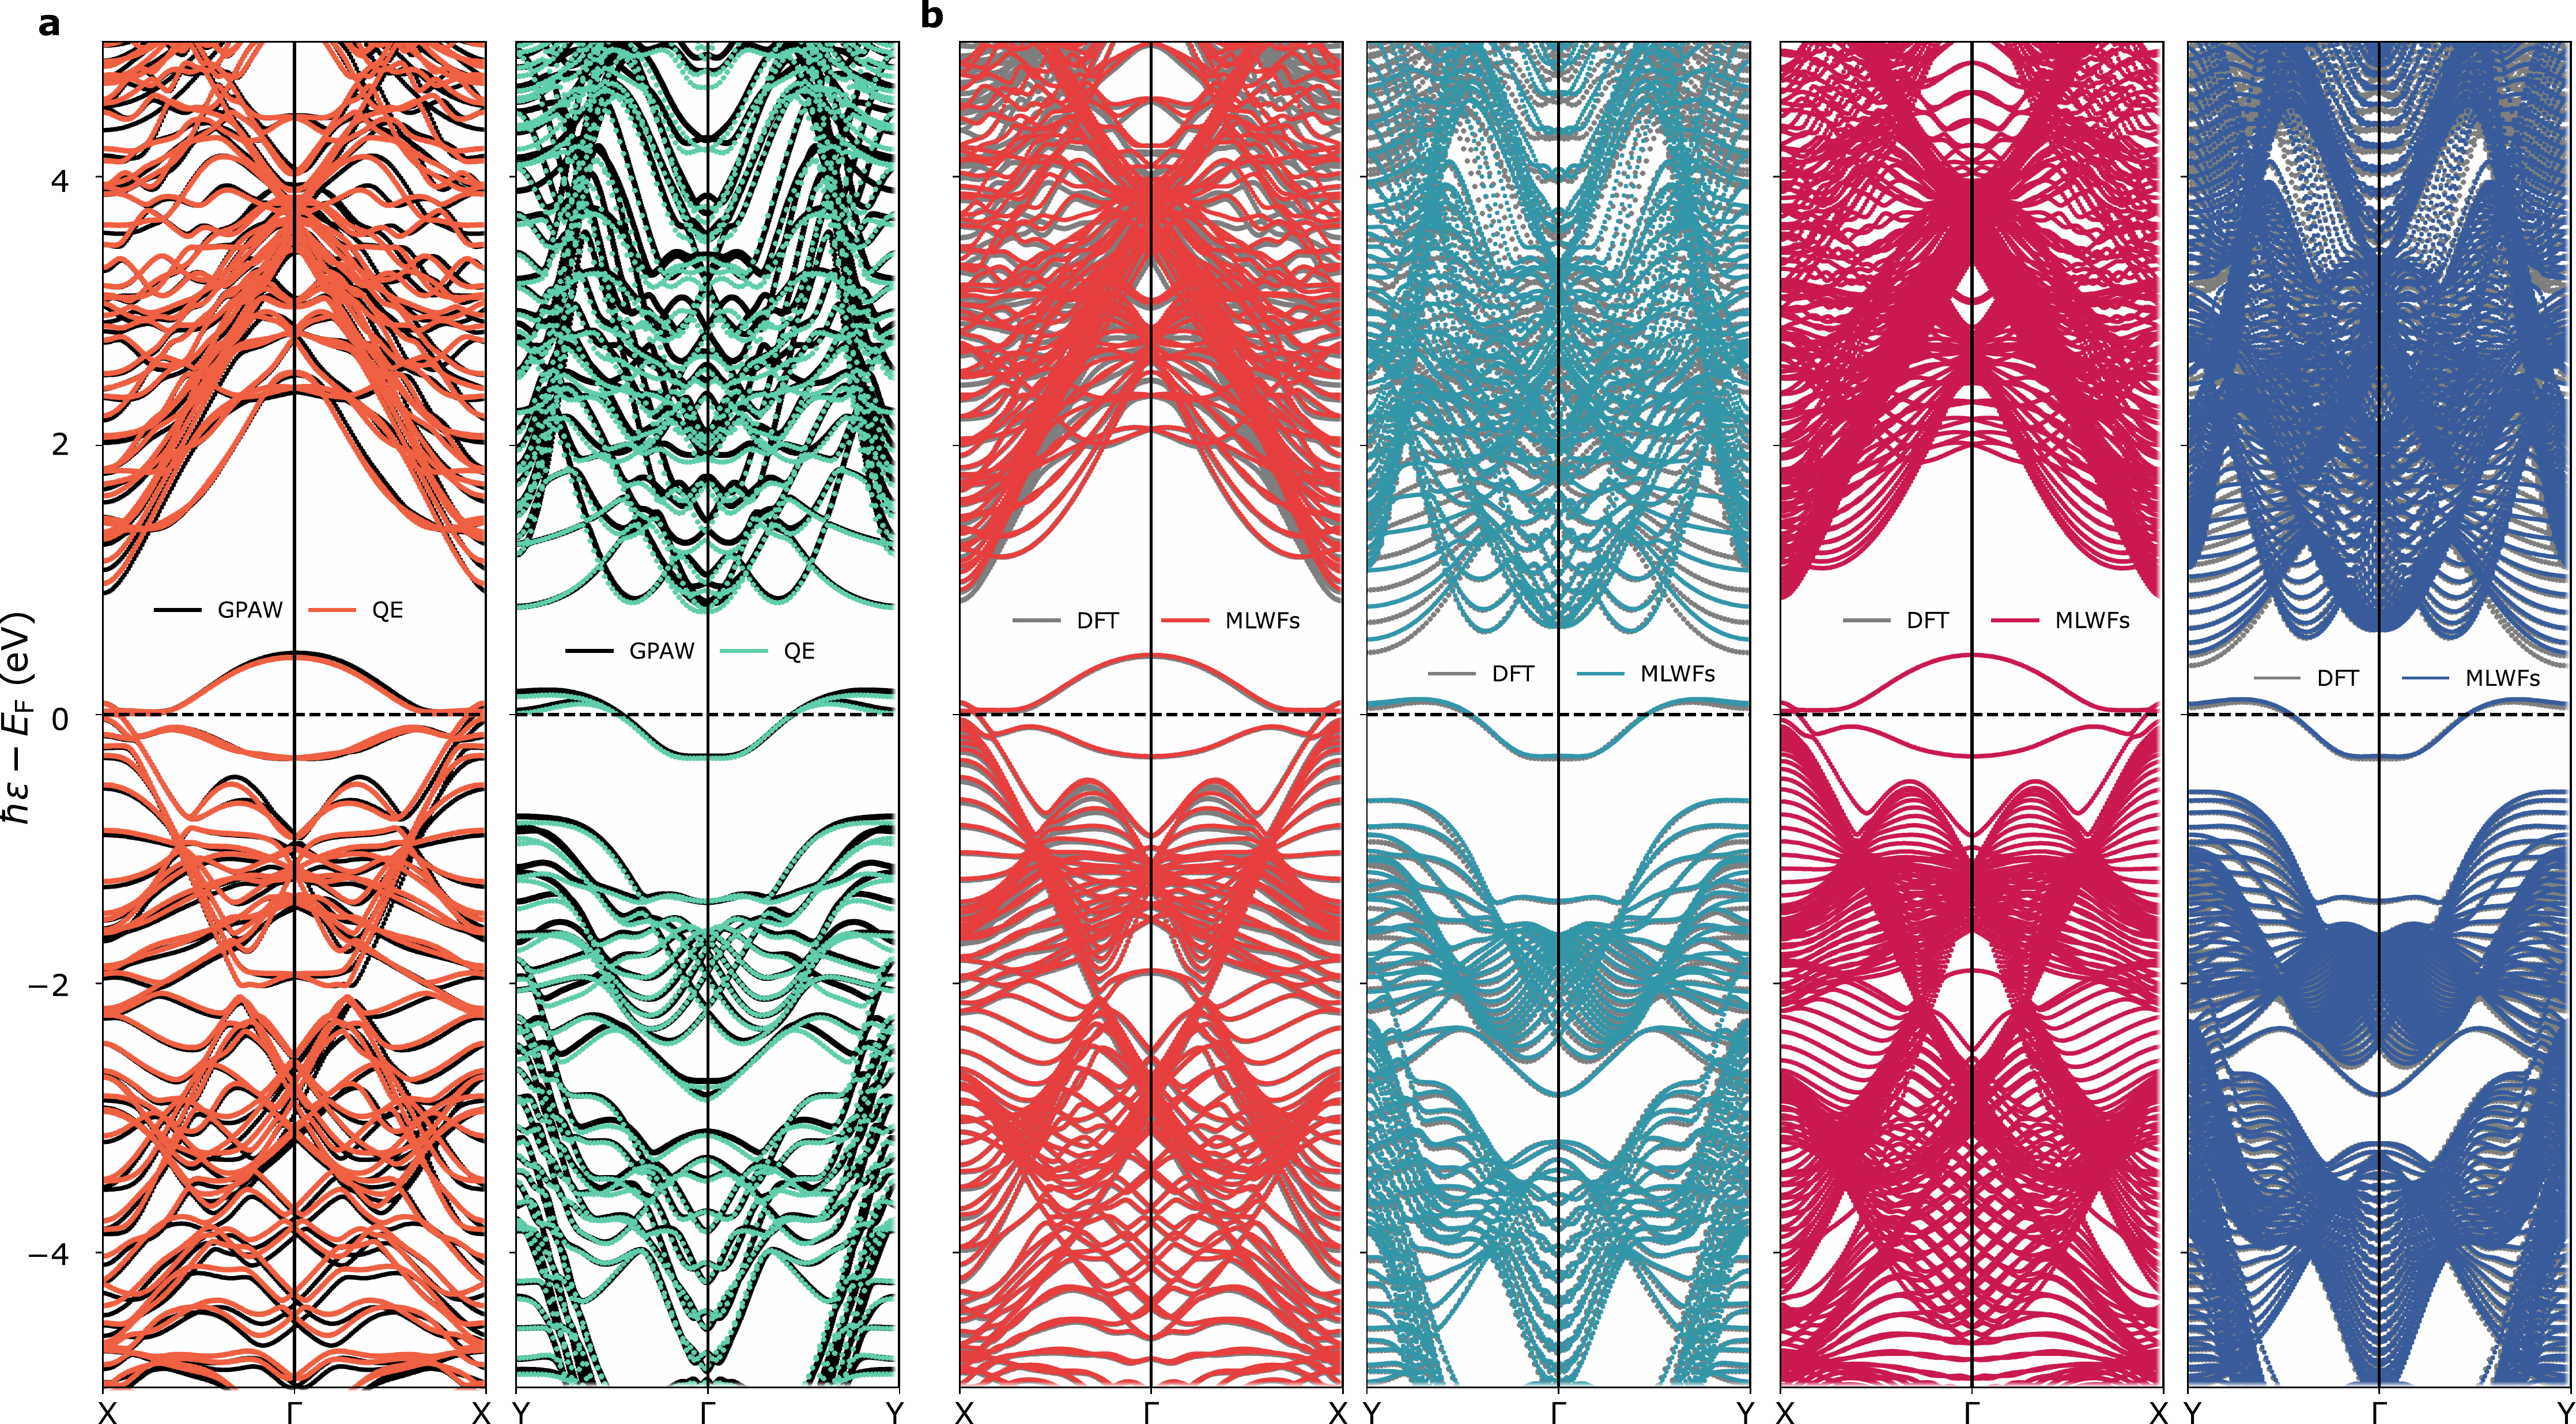}
    \caption{\textbf{Electronic band structure in phosphorene nanoribbons.} The Wannier tight-binding (WTB) Hamiltonians are constructed from ab-initio electronic band structure calculations performed using the Quantum Espresso (QE) code \cite{QE}, which forms the basis for optical response calculations performed at the level of the random-phase approximation (RPA). In Fig.\ 1 of the main text we compare the linear optical response obtained from WTB-RPA simulations with that obtained directly from the GPAW code \cite{mortensen2005real,enkovaara2010electronic}, from which the electronic band structure is computed independently from first-principles for the smallest armchair (AC) and zigzag (ZZ) phosphorene nanoribbons (PNRs) considered. In panel \textbf{a} we present the electronic band structures of the smallest PNRs considered in the main text, as obtained using GPAW (black curves) and QE (colored curves) codes for AC and ZZ ribbons of indicated widths $W$. Panel \textbf{b} shows the band structures obtained directly from QE for larger ribbons (black curves), which are reproduced by the bands obtained upon diagonalization of the constructed WTB Hamiltonian.}
    \label{fig:DFT_codes}
\end{figure}

\clearpage

\begin{figure}[t]
    \centering
    \includegraphics[width=0.75\textwidth]{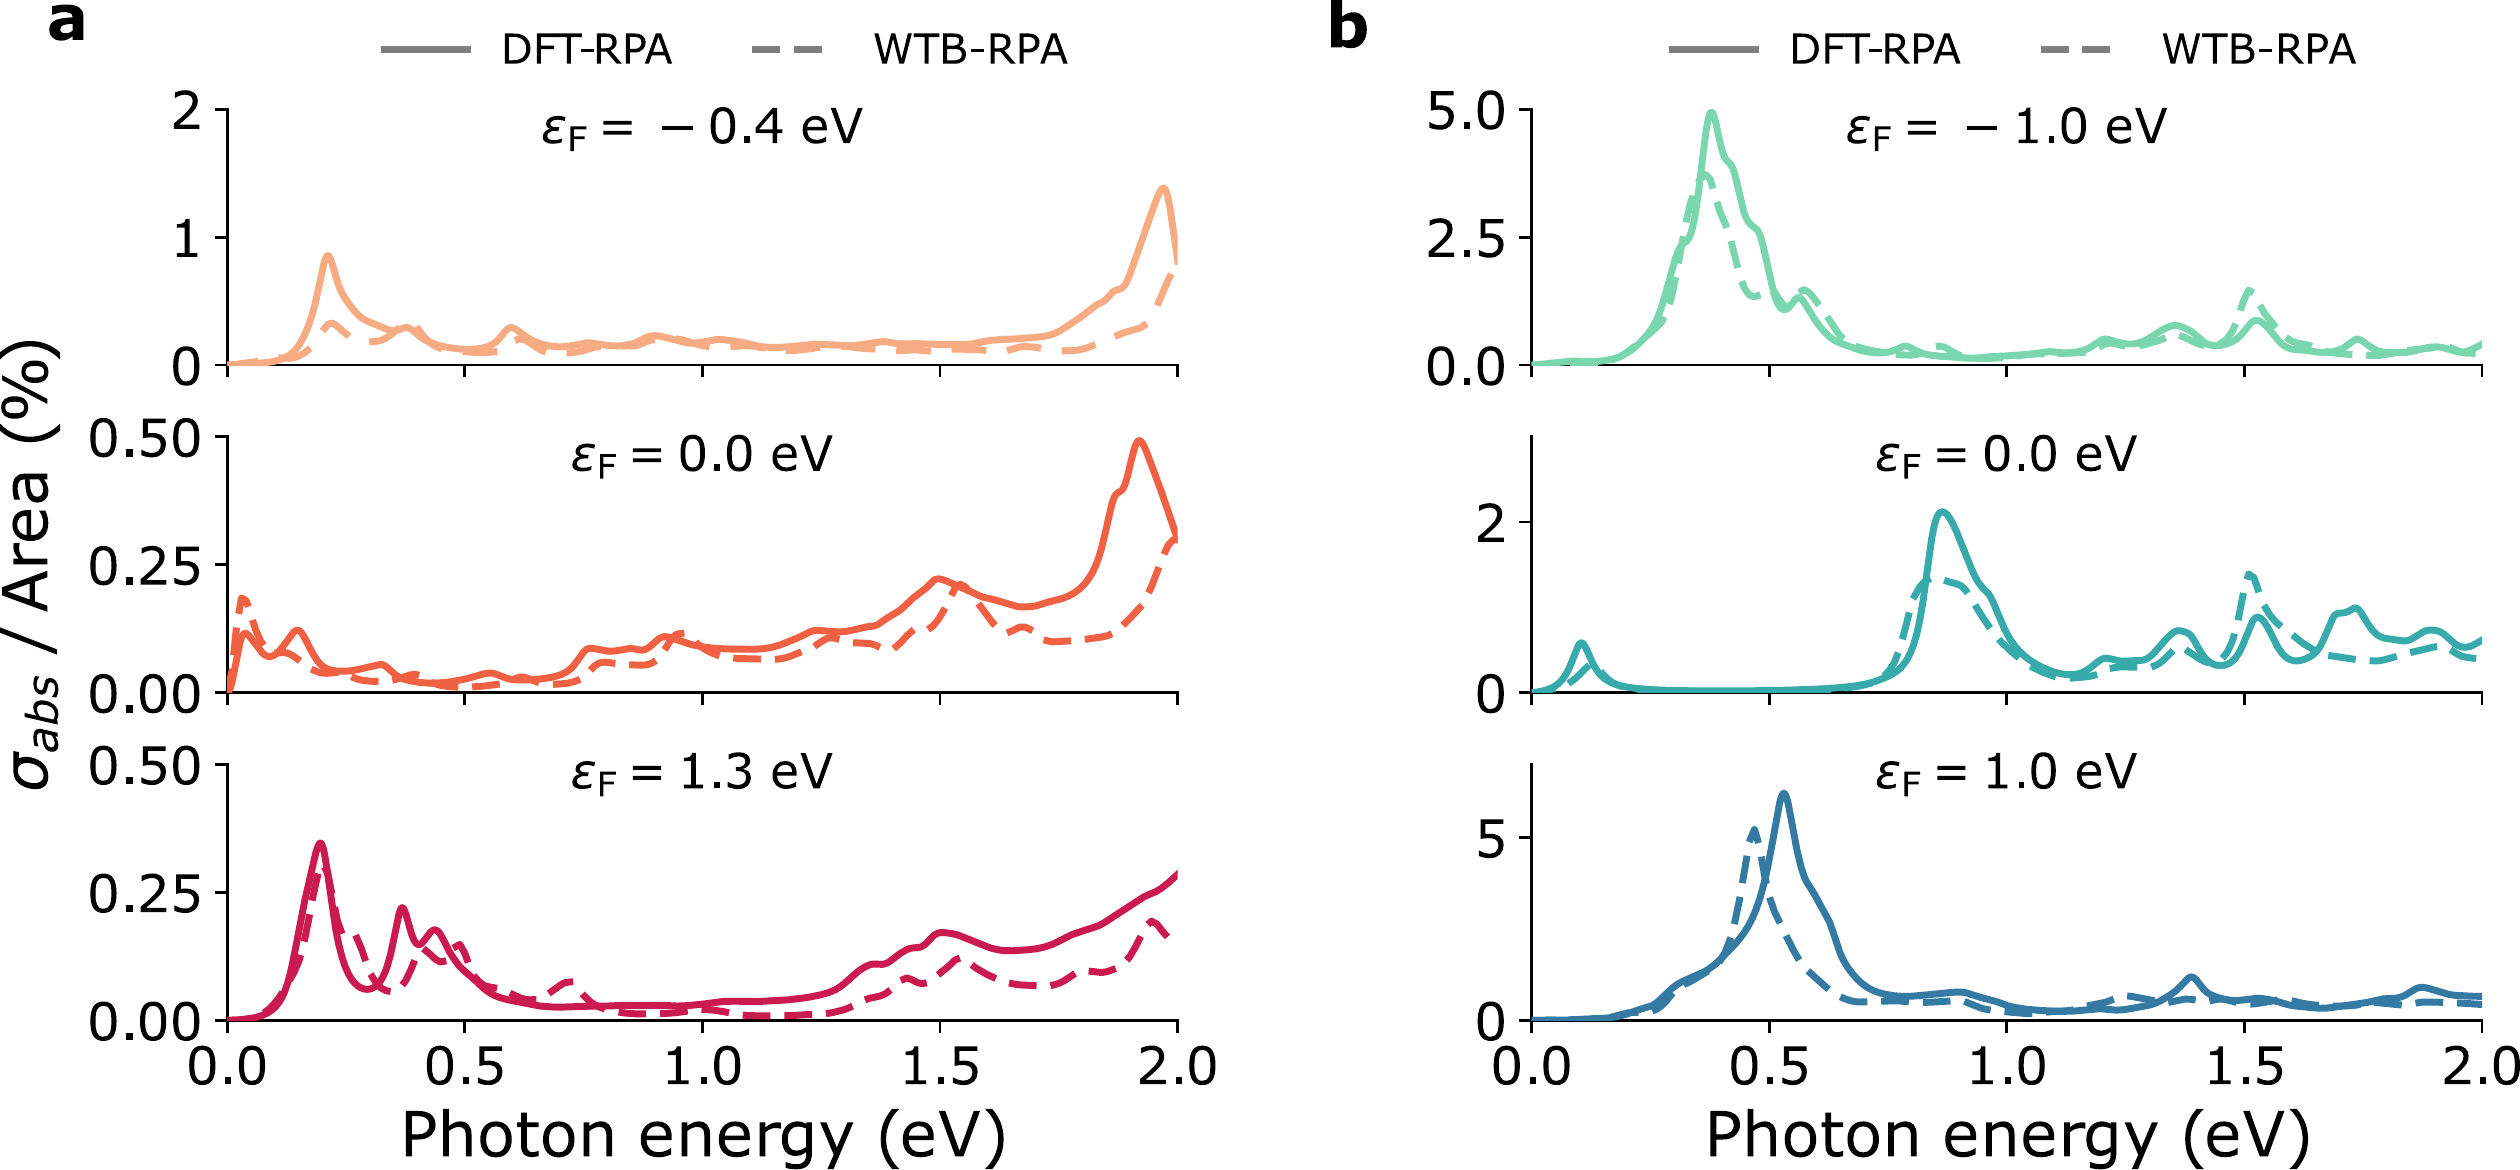}
    \caption{\textbf{Linear optical response of phosphorene nanoribbons neglecting Coulomb interactions.} We present the absorption cross-section per unit area of the phosphorene nanoribbons considered in Fig.\ 1 of the main text but neglecting electron-electron interactions in the optical response. Results are presented for \textbf{a} armchair edge-terminated ribbons of $W=2.6$\,nm width and \textbf{b} zigzag edge-terminated ribbons of $W=2.8$\,nm width at doping levels indicated by the corresponding Fermi energy $E_{\rm F}$, where results from the Wannier tight-binding model are compared to those obtained directly from DFT optical response calculations.}
    \label{fig:noC}
\end{figure}

%%%%%%%%%%%%%%%%%%%%%%%%%%%%%%%%%%%%%%%%%%%%%%%%%%%%%%%%%%%%%%%%%%%%%%%%%%%%%%%
%\bibliographystyle{apsrev4-2}
%\bibliography{refs}

%apsrev4-2.bst 2019-01-14 (MD) hand-edited version of apsrev4-1.bst
%Control: key (0)
%Control: author (72) initials jnrlst
%Control: editor formatted (1) identically to author
%Control: production of article title (-1) disabled
%Control: page (0) single
%Control: year (1) truncated
%Control: production of eprint (0) enabled
%

\end{document}
